# Supplementary material for: Multi-state quantum simulations via model-space quantum imaginary time evolution
Source: arXiv:2206.04494 ancillary file (2023-09-29)
Supplement: Supplementary file 1 [file SI.pdf]

# Supporting Information for “Multi-state quantum simulations via model-space quantum imaginary time evolution”

Takashi Tsuchimochi\*

*Graduate School of System Informatics,  
Kobe University, 1-1 Rokkodai-cho,  
Nada-ku, Kobe, Hyogo 657-8501 Japan and  
Japan Science and Technology Agency (JST),  
Precursory Research for Embryonic Science and Technology (PRESTO),  
4-1-8 Honcho Kawaguchi, Saitama 332-0012 Japan*

Yoohee Ryo

*Graduate School of Science, Technology,  
and Innovation, Kobe University, 1-1 Rokkodai-cho,  
Nada-ku, Kobe, Hyogo 657-8501 Japan*

Seiichiro L. Ten-no

*Graduate School of System Informatics,  
Kobe University, 1-1 Rokkodai-cho,  
Nada-ku, Kobe, Hyogo 657-8501 Japan*

---

\* [tsuchimochi@gmail.com](mailto:tsuchimochi@gmail.com)

## QITE

In QITE, the imaginary time evolution of the state  $|\Phi\rangle$  is Trotterized and the following unitary approximation was applied[1],

$$|\Phi'\rangle = \frac{1}{\sqrt{c}} e^{-\Delta\beta\hat{H}} |\Phi\rangle \approx e^{-i\Delta\beta\hat{A}} |\Phi\rangle \quad (\text{S1})$$

where

$$c = \langle\Phi|e^{-2\Delta\beta\hat{H}}|\Phi\rangle \quad (\text{S2})$$

is the squared norm, and  $\hat{A}$  is defined as

$$\hat{A} = \sum_{\mu} a_{\mu} \hat{\sigma}_{\mu} \quad (\text{S3})$$

with Pauli strings  $\hat{\sigma}_{\mu}$ .

The real coefficients  $a_{\mu}$  are determined by minimizing the following quantity to the second order of  $\Delta\beta$ [2],

$$F(\mathbf{a}) = \left\| \frac{1}{\sqrt{c}} e^{-\Delta\beta\hat{H}} |\Phi\rangle - e^{-i\Delta\beta\hat{A}} |\Phi\rangle \right\|^2 \quad (\text{S4})$$

yielding

$$M_{\mu\nu} = 2\text{Re}\langle\Phi|\hat{\sigma}_{\mu}\hat{\sigma}_{\nu}|\Phi\rangle \quad (\text{S5})$$

$$b_{\mu} = \text{Im}\langle\Phi|[\hat{H}, \hat{\sigma}_{\mu}]|\Phi\rangle \quad (\text{S6})$$

## Fermionic-QITE

Fermionic-QITE uses anti-Hermitian fermionic operators to construct the chemistry-inspired  $\hat{A}$ ,

$$\hat{A} = \hat{A}_1 + \hat{A}_2 + \dots \quad (\text{S7a})$$

$$\hat{A}_1 = \sum_{pq} t_{pq} (c_p^{\dagger} c_q - c_q^{\dagger} c_p) \quad (\text{S7b})$$

$$\hat{A}_2 = \frac{1}{4} \sum_{pqrs} t_{pqrs} (c_p^{\dagger} c_q^{\dagger} c_s c_r - c_r^{\dagger} c_s^{\dagger} c_q c_p) \quad (\text{S7c})$$

where  $\mathbf{t}$  is purely imaginary.  $\hat{A}_k$  comprises the  $k$ -rank excitation and de-excitation operators, and Eq. (S7) is appropriately transformed to the qubit basis as Eq. (S7). Truncated after

$\hat{A}_3$ ,  $\hat{A} = \hat{A}_1 + \hat{A}_2$  is known as unitary coupled-cluster with generalized singles and doubles (UCCGSD) and defines “UCCGSD-based QITE” after a certain transformation to the qubit representation.

### Derivation of the working equations of MSQITE and MS-QLanczos

Our goal is to find the approximation

$$|\Phi_I^{(\ell+1)}\rangle = \sum_J d_{IJ} e^{-\Delta\beta(\hat{H}-E_J)} |\Phi_J^{(\ell)}\rangle \approx e^{-i\Delta\beta\hat{A}} |\Phi_I^{(\ell)}\rangle. \quad (\text{S8})$$

To obtain the equation for MSQITE, we minimize  $F^I$ , i.e., the distance between the left and right hand sides of Eq. (S8), noting that it is also crucial to take into account the dependence of  $\mathbf{d}$  on  $\Delta\beta$ . As described in the main text,  $\mathbf{d}$  is determined by orthonormalizing  $\tilde{S}_{IJ} = \langle \Phi_I | e^{-\Delta\beta(\hat{H}-E_I)} e^{-\Delta\beta(\hat{H}-E_J)} | \Phi_J \rangle$ . Because  $\tilde{S}_{IJ} \rightarrow \delta_{IJ}$  as  $\Delta\beta \rightarrow 0$ , we also have  $d_{IJ} \rightarrow \delta_{IJ}$  (see the Methods section in the main text). Note that, for the state-specific problem, the state basis  $\{|\Phi_I^{(\ell)}\rangle\}$  are not necessarily orthogonal to each other because they are evolved by different unitaries. Therefore we need to assume or impose the same limit for  $d_{JI}$ , because otherwise Eq. (S8) would become obviously contradictory at  $\Delta\beta = 0$ . The condition can be strictly imposed by defining  $\mathbf{d}$  from  $\tilde{\mathbf{S}}$  in the transformed model space so that  $\mathbf{S} = \mathbf{1}$ , which is then back-transformed to the current model space. Namely, one may have  $\mathbf{d}$  by the Löwdin symmetric orthonormalization of the following overlap:

$$\tilde{S}'_{IJ} = \mathbf{d}' \tilde{\mathbf{S}} \mathbf{d}' \quad (\text{S9})$$

where  $\mathbf{d}'$  itself is the Löwdin symmetric orthonormalization coefficients of  $\mathbf{S}$ , which is independent of  $\Delta\beta$  (for the purpose of expanding  $F^I$ ). However, our numerical tests revealed that this procedure does not affect the convergence behavior, and hence we simply use the  $\mathbf{d}$  defined in the main text and assume that the limit  $d_{IJ} \rightarrow \delta_{IJ}$  holds.

Then, it is convenient to write

$$d_{JI} = \delta_{JI} + \Delta\beta \Delta d_{JI} + O(\Delta\beta^2) \quad (\text{S10})$$

and let us consider the expansion of  $F^I$  up to the second-order in  $\Delta\beta$  as follows:

$$\begin{aligned}
F^I(\mathbf{a}^I) &= \left\| \sum_J d_{JI} e^{-\Delta\beta(\hat{H}-E_J)} |\Phi_J^{(\ell)}\rangle - e^{-i\Delta\beta\hat{A}^I} |\Phi_I^{(\ell)}\rangle \right\|^2 \\
&= 2 - \sum_J d_{JI} \left( \langle \Phi_J^{(\ell)} | e^{-\Delta\beta(\hat{H}-E_J)} e^{-i\Delta\beta\hat{A}^I} |\Phi_I^{(\ell)}\rangle + \langle \Phi_I^{(\ell)} | e^{i\Delta\beta\hat{A}^I} e^{-\Delta\beta(\hat{H}-E_J)} |\Phi_J^{(\ell)}\rangle \right) \\
&= 2 - \sum_J (\delta_{JI} + \Delta\beta\Delta d_{JI} + O(\Delta\beta^2)) \left( \right. \\
&\quad \langle \Phi_J^{(\ell)} | (1 - \Delta\beta(\hat{H} - E_J) + \frac{1}{2}\Delta\beta^2(\hat{H} - E_J)^2)(1 - i\Delta\beta\hat{A}^I - \frac{1}{2}\Delta\beta^2(\hat{A}^I)^2) |\Phi_I^{(\ell)}\rangle \\
&\quad \left. + \langle \Phi_I^{(\ell)} | (1 + i\Delta\beta\hat{A}^{I\dagger} - \frac{1}{2}\Delta\beta^2(\hat{A}^I)^2)(1 - \Delta\beta(\hat{H} - E_J) + \frac{1}{2}\Delta\beta^2(\hat{H} - E_J)^2) |\Phi_J^{(\ell)}\rangle \right) + O(\Delta\beta^3) \\
&= \text{const.} + \Delta\beta \sum_J (\delta_{JI} + \Delta\beta\Delta d_{JI}) \left( i\langle \Phi_J^{(\ell)} | \hat{A}^I | \Phi_I^{(\ell)}\rangle - i\langle \Phi_I^{(\ell)} | \hat{A}^I | \Phi_J^{(\ell)}\rangle \right) \\
&\quad + \Delta\beta^2 \sum_J \delta_{JI} \left( \langle \Phi_J^{(\ell)} | \left( -i(\hat{H} - E_J)\hat{A}^I + \frac{1}{2}(\hat{A}^I)^2 \right) | \Phi_I^{(\ell)}\rangle \right. \\
&\quad \left. + \langle \Phi_I^{(\ell)} | \left( i\hat{A}^I(\hat{H} - E_J) + \frac{1}{2}(\hat{A}^I)^2 \right) | \Phi_J^{(\ell)}\rangle \right) + O(\Delta\beta^3) \tag{S11}
\end{aligned}$$

$$\begin{aligned}
&= \text{const.} + \Delta\beta^2 \left( \langle \Phi_I^{(\ell)} | (\hat{A}^I)^2 | \Phi_I^{(\ell)}\rangle - i\langle \Phi_I^{(\ell)} | [\hat{H}, \hat{A}^I] | \Phi_I^{(\ell)}\rangle \right. \\
&\quad \left. + i \sum_J \Delta d_{JI} \left( \langle \Phi_J^{(\ell)} | \hat{A}^I | \Phi_I^{(\ell)}\rangle - \langle \Phi_I^{(\ell)} | \hat{A}^I | \Phi_J^{(\ell)}\rangle \right) \right) + O(\Delta\beta^3) \tag{S12}
\end{aligned}$$

Perhaps surprisingly, the terms in the parenthesis do not have an explicit energy dependence; however, the constant term does. Also, it is important to introduce  $E_I$  for  $\Delta d_{JI}$  to be small so that Eq. (S10) is valid. The additional third term in the parenthesis maintains the orthogonality. We approximate  $\Delta d_{JI}$  by using Eq. (S10),

$$\Delta d_{JI} \approx \frac{d_{JI} - \delta_{JI}}{\Delta\beta} \tag{S13}$$

and arrive at

$$\begin{aligned}
f^I(\mathbf{a}^I) &= \langle \Phi_I^{(\ell)} | (\hat{A}^I)^2 | \Phi_I^{(\ell)}\rangle + \text{Im}\langle \Phi_I^{(\ell)} | [\hat{H}, \hat{A}^I] | \Phi_I^{(\ell)}\rangle \\
&\quad + \frac{2}{\Delta\beta} \sum_J d_{JI} \text{Im}\langle \Phi_I^{(\ell)} | \hat{A}^I | \Phi_J^{(\ell)}\rangle. \tag{S14}
\end{aligned}$$

We also show the derivation of the matrix element required in MS-QLanczos for clarity. For the overlap matrix,

$$\begin{aligned}
\mathcal{S}_{I(\ell), J(\ell')} &\equiv \langle \Phi_I^{(\ell)} | \Phi_J^{(\ell')} \rangle \\
&= \sum_{KL} \left( \tilde{\mathbf{d}}^{(0)} \tilde{\mathbf{d}}^{(1)} \dots \tilde{\mathbf{d}}^{(\ell-1)} \right)_{KI} \left( \tilde{\mathbf{d}}^{(0)} \tilde{\mathbf{d}}^{(1)} \dots \tilde{\mathbf{d}}^{(\ell'-1)} \right)_{LJ} \underbrace{\langle \Phi_K^{(0)} | e^{-\ell \Delta \beta (\hat{H} - E_0)} e^{-\ell' \Delta \beta (\hat{H} - E_0)} | \Phi_L^{(0)} \rangle}_{\langle \Phi_K^{(0)} | e^{-(\ell+\ell')/2 \Delta \beta (\hat{H} - E_0)} e^{-(\ell+\ell')/2 \Delta \beta (\hat{H} - E_0)} | \Phi_L^{(0)} \rangle} \\
&= \sum_{KLMN} \left( \tilde{\mathbf{d}}^{(0)} \tilde{\mathbf{d}}^{(1)} \dots \tilde{\mathbf{d}}^{(\frac{\ell+\ell'}{2}-1)} \right)_{KM} \left( \tilde{\mathbf{d}}^{(\frac{\ell+\ell'}{2})} \dots \tilde{\mathbf{d}}^{(\ell-1)} \right)_{MI} \times \\
&\quad \left( \tilde{\mathbf{d}}^{(0)} \tilde{\mathbf{d}}^{(1)} \dots \tilde{\mathbf{d}}^{(\ell'-1)} \tilde{\mathbf{d}}^{(\ell')} \dots \tilde{\mathbf{d}}^{(\frac{\ell+\ell'}{2}-1)} \right)_{LN} \left( (\tilde{\mathbf{d}}^{(\frac{\ell+\ell'}{2}-1)})^{-1} \dots (\tilde{\mathbf{d}}^{(\ell')})^{-1} \right)_{NJ} \times \\
&\quad \langle \Phi_K^{(0)} | e^{-\frac{\ell+\ell'}{2} \Delta \beta (\hat{H} - E_0)} e^{-\frac{\ell+\ell'}{2} \Delta \beta (\hat{H} - E_0)} | \Phi_L^{(0)} \rangle \\
&= \sum_{MN} \left( \tilde{\mathbf{d}}^{(\frac{\ell+\ell'}{2})} \dots \tilde{\mathbf{d}}^{(\ell-1)} \right)_{MI} \left( (\tilde{\mathbf{d}}^{(\frac{\ell+\ell'}{2}-1)})^{-1} \dots (\tilde{\mathbf{d}}^{(\ell')})^{-1} \right)_{NJ} \underbrace{\langle \Phi_M^{(\frac{\ell+\ell'}{2})} | \Phi_N^{(\frac{\ell+\ell'}{2})} \rangle}_{S_{MN}^{(\frac{\ell+\ell'}{2})}} \\
&= \sum_{MN} \left( \tilde{\mathbf{d}}^{(\frac{\ell+\ell'}{2})} \dots \tilde{\mathbf{d}}^{(\ell-1)} \right)_{MI} \left( \tilde{\mathbf{d}}^{(\ell')} \dots \tilde{\mathbf{d}}^{(\frac{\ell+\ell'}{2}-1)} \right)_{NJ}^{-1} S_{MN}^{(\frac{\ell+\ell'}{2})} \\
&= \left[ \left( \mathbf{D}^{(\frac{\ell+\ell'}{2} \rightarrow \ell-1)} \right)^\top \mathbf{S}^{(\frac{\ell+\ell'}{2})} \left( \mathbf{D}^{(\ell' \rightarrow \frac{\ell+\ell'}{2}-1)} \right)^{-1} \right]_{IJ}. \tag{S15}
\end{aligned}$$

The matrix elements for the effective Hamiltonian and other operators (that commute with  $\hat{H}$  such as  $\hat{S}^2$ ) are derived similarly.

### Supplementary data

We provide the coefficients of eigenstates for BeH<sub>2</sub> obtained by the exact diagonalization in Table S1.

- 
- [1] M. Motta, C. Sun, A. T. K. Tan, M. J. O'Rourke, E. Ye, A. J. Minnich, F. G. S. L. Brandão, and G. K.-L. Chan, *Nat. Phys.* **16**, 205 (2020).
- [2] T. Tsuchimochi, Y. Ryo, and S. L. Ten-no, (2022), [arXiv:2205.01983 \[quant-ph\]](#).

TABLE S1. Coefficients of exact eigenstates for BeH<sub>2</sub>.

| Configuration            | $XA_g$  | $2A_g$  | $3A_g$  | $4A_g$  |
|--------------------------|---------|---------|---------|---------|
| $ 000000001111\rangle^a$ | 0.9859  | 0.0678  | 0.0000  | -0.0086 |
| $ 000000011011\rangle$   | 0.0000  | 0.0000  | 0.0000  | 0.0000  |
| $ 000000100111\rangle$   | 0.0000  | 0.0000  | 0.0000  | 0.0000  |
| $ 000000110011\rangle^b$ | 0.0004  | -0.3357 | 0.4987  | 0.4113  |
| $ 000000111100\rangle$   | -0.0558 | 0.3785  | -0.4663 | -0.2003 |
| $ 000001001011\rangle$   | 0.0000  | 0.0000  | 0.0000  | 0.0000  |
| $ 000010000111\rangle$   | 0.0000  | 0.0000  | 0.0000  | 0.0000  |
| $ 000011000011\rangle^c$ | 0.0004  | -0.3357 | -0.4987 | 0.4113  |
| $ 000011001100\rangle$   | -0.0558 | 0.3785  | 0.4663  | -0.2003 |
| $ 000100001110\rangle$   | -0.0115 | 0.4004  | 0.0000  | 0.5211  |
| $ 000100101001\rangle$   | 0.0000  | 0.0000  | 0.0000  | 0.0000  |
| $ 000100110010\rangle$   | 0.0068  | -0.0977 | 0.1115  | 0.0533  |
| $ 000111000010\rangle$   | 0.0068  | -0.0977 | -0.1115 | 0.0533  |
| $ 001000001101\rangle$   | 0.0115  | -0.4004 | 0.0000  | -0.5211 |
| $ 001000010110\rangle$   | 0.0000  | 0.0000  | 0.0000  | 0.0000  |
| $ 001000110001\rangle$   | -0.0068 | 0.0977  | -0.1115 | -0.0533 |
| $ 001011000001\rangle$   | -0.0068 | 0.0977  | 0.1115  | -0.0533 |
| $ 001100000011\rangle$   | -0.0794 | 0.2671  | 0.0000  | 0.1143  |
| $ 001100001100\rangle$   | -0.0587 | -0.1425 | 0.0000  | -0.0236 |

<sup>a</sup> Configuration (i) of Fig. 2.

<sup>b</sup> Configuration (ii) of Fig. 2.

<sup>c</sup> Configuration (iii) of Fig. 2.
